# Supplementary material for: AMR-Transformer: Enabling Efficient Long-range Interaction for Complex Neural Fluid Simulation
Source: arXiv:2503.10257 source file (2025-03-13)
Supplement: Supplementary file 2 [file Appendix.tex]

\section{Appendix}
\label{sec:appendix}

\subsection{Shockwave Description}
\label{sec:shockwave_appendix}
    We utilize a two-dimensional (2D) Riemann problem, specifically Configuration 3 from Kurganov and Tadmor~\cite{kurganov2002solution}, to generate a new dataset aimed at evaluating the performance of our proposed Adaptive Mesh Refinement (AMR)-Transformer pipeline and other baselines. The initial conditions for the problem are defined as:
    \begin{equation}
    \resizebox{\hsize}{!}{$
    \left(\rho, u, v, p \right) = \begin{cases}
    (1.5, 0, 0, 1.5), & \text{if} \quad x > 0.5, y > 0.5, \\
    (0.5323, 1.206, 0, 0.3), & \text{if} \quad x < 0.5, y > 0.5, \\
    (0.138, 1.206, 1.206, 0.029), & \text{if} \quad x < 0.5, y < 0.5, \\
    (0.5323, 0, 1.206, 0.3), & \text{if} \quad x > 0.5, y < 0.5.
    \end{cases}
    $}
    \end{equation}
    Here, $\rho$ denotes the density, $u$ and $v$ are the velocity components in the $x$ and $y$ directions respectively, and $p$ is the pressure. The computational domain is $[0,1]^2$, and Neumann boundary conditions are applied on all sides. Simulations are conducted up to a final time of $t = 0.3$. To generate a robust dataset, random symmetry-preserving perturbations with a maximum deviation of $20\%$ are applied to the initial conditions, resulting in 10 unique unsteady simulation instances. Each simulation is represented by time-evolving snapshots of the solutions, providing a comprehensive view of the system’s temporal and spatial dynamics.
    
    The dataset size is $128 \times 128$, which is four times larger than the CFDBench datasets with $64 \times 64$. Each cell contains the velocity components $u$, $v$, pressure $p$, and density $\rho$, allowing for a more detailed representation of the flow features. All simulations employ the WENO5-Z scheme~\cite{borges2008improved}, well-regarded for accurately capturing high-gradient regions and minimizing numerical diffusion in the presence of strong shocks.
    
    Compared to existing benchmark cases like the CFDBench cylinder and cavity flows, our dataset offers significant advantages. The cylinder flow is characterized by simple periodic vortex shedding with large coherent structures, lacking small-scale features and complex unsteady evolution. Similarly, the cavity flow involves coherent vortices in a steady-state problem, lacking temporal complexity. In contrast, the dataset generated from the 2D Riemann problem contains strong shock waves with sharp discontinuities and a complex time evolution of small-scale vortex structures, presenting a multiscale flow structure.
    
    This dataset is uniquely suited to evaluating the performance of the proposed AMR-transformer framework, which is designed to handle complex multiscale information efficiently. Specifically, it allows us to assess the framework's ability to accurately identify regions with high gradients for mesh refinement, thereby increasing local accuracy. The presence of both discontinuities (shock waves) and small-scale vortex structures near the shocks introduces multiscale flow features that challenge traditional methods. Our dataset's complexity in flow structures is crucial for testing and demonstrating the precision and effectiveness of the AMR-Transformer framework in handling such intricate phenomena.

\subsection{3D Sinusoidal Positional Encoding}
\label{sec:pos_encoding_appendix}
    The 3D sinusoidal positional encoding used in our model introduces unique encodings for each spatial coordinate \(x\), \(y\), and depth \(d\). These encodings are then added to the upsampled feature vectors of dimensionality \(d_{\text{model}}\), providing spatial context for the AMR-Transformer. The encoding dimensions are split equally, with \(d_{\text{model}}\) divided into three parts allocated to \(x\), \(y\), and \(d\).

    For each coordinate (\(\text{coord}\)), the positional encoding is calculated as:
    \[
    \text{pe}_{\text{coord}} = \left[ \sin\left(\text{coord} \times \text{div\_term}\right), \cos\left(\text{coord} \times \text{div\_term}\right) \right],
    \]
    where \(\text{div\_term} = \exp\left(\frac{-\log(10000) \cdot i}{d_{\text{coord}}}\right)\), and \(i\) indexes over the dimension range \(d_{\text{coord}}\) allocated to each spatial component. This scaling controls the frequency of the sinusoidal functions relative to \(d_{\text{model}}\).
    
    Each position component \(x\), \(y\), and \(d\) is flattened into a 1D vector and encoded independently. The final positional encoding vector \(\text{pos\_encoding}\) is constructed by concatenating these encodings and reshaping back to \((b, n, d_{\text{model}})\), where \(b\) is the batch size and \(n\) is the number of patches:
    \[
    \text{pos\_encoding} = [\text{pe}_x, \text{pe}_y, \text{pe}_d].
    \]
    This positional encoding is then added element-wise to the upsampled feature vectors, embedding spatial information directly into the model’s input tokens.

% \subsection{Threshold Settings and Condition Evaluation Details}
% \label{sec:threshold_and_condition_appendix}

% \subsection{Model Details}
% \label{sec:model_details}
